# Supplementary material for: Momentum Centering and Asynchronous Update for Adaptive Gradient Methods
Source: arXiv:2110.05454 source file (2021-12-01)
Supplement: Supplementary file 1 [file appendix_sec_convex_convergence.tex]

\section{Convergence analysis for online convex optimization}
\subsection{Problem definition}
The problem for online convex optimization is
\begin{equation}
    \operatorname{min}_{x \in \mathcal{F}} \sum_{t=1}^T f_t (x)
    \label{eq:convex_problem}
\end{equation}
where $\mathcal{F}$ is a convex feasible set, $f_t(x)$ is a convex function for each $t$. Note that $f_i$ and $f_j$ could be different functions, as long as they are both convex.
\subsection{Convergence analysis of Async-optimizers for online convex optimization}

\begin{lemma} \label{lemma:non-expansive}
Let $A \in \mathbb{R}^{d \times d}$ be a symmetric, positive definite matrix, let $\mathcal{F}$ be a convex set, denote the weighted projection $\mathcal{P}_{\mathcal{F}}^A(z)$ of $z$ onto convex set $\mathcal{F}$ as
\begin{equation}
    \mathcal{P}_{\mathcal{F}}^A(z) = \operatorname{argmin}_{x \in \mathcal{F}} \Big \langle x-z, A(x-z) \Big \rangle \coloneqq \operatorname{argmin}_{x \in \mathcal{F}} \vert \vert x-z \vert \vert_A^2 
\end{equation}
then 
\begin{equation}
    \vert \vert \mathcal{P}_{\mathcal{F}}^A(x) - \mathcal{P}_{\mathcal{F}}^A(y) \vert \vert_A \leq \vert \vert x - y \vert \vert_A 
\end{equation}
\end{lemma}
\begin{proof}
See \cite{mcmahan2010adaptive}.
\end{proof}
\begin{theorem}[Thm 3.4 in the main paper]
\label{thm:convex_bgrad_converge}
For the problem defined by Eq.~\eqref{eq:convex_problem}, suppose the optimal solution is $x^*$, suppose the convex feasible set $\mathcal{F}$ has bounded diameter $D$ (e.g. $\vert \vert x - y \vert \vert<D, \forall x, y \in \mathcal{F}$), $0<\beta_1 < 1, 0<\beta_2 < 1$, also assume $H_{t+1} \leq H_{t}$ element-wise (this can be achieved by tracking element-wise maximum of the second moment as in AMSGrad) and $\vert \vert g_t \vert  \vert_{\infty} \leq M_g$, with learning rate schedule as
\begin{equation}
\alpha_t = \alpha_0 t^{-\eta},\ \  \eta \in [0.5, 1)
\end{equation}
assume $H_t$ is both lower-bounded and upper-bounded, there exist positive constants $C_l, C_u$ $s.t.$
\begin{equation}
C_l I \preceq H_t \preceq C_u I, \ \ \forall t 
\end{equation}
where the notation $A \preceq B$ means the matrix $B-A$ is positive-semidefinite.
the sequence is generated by 
\begin{equation}
    x_{t+1} = \mathcal{P}_\mathcal{F}^{\mathbf{1}} \Big( x_t - \alpha_t H_t g_t \Big)
\end{equation}
where $\mathcal{P}_\mathcal{F}$ represents the projection onto convex set $\mathcal{F}$.
Then we have
\begin{equation}
    \frac{1}{T} \sum_{t=1}^T \Big( f_t(x_t) - f_t(x^*) \Big) \leq \frac{1}{C_l} \frac{D^2}{2 \alpha_0} T^{\eta-1}+C_u \frac{M_g^2 \alpha_0}{2(1-\eta)}T^{-\eta} + O(T^{-1})
\end{equation}
\end{theorem}
\begin{proof}
By Lemma.~\ref{lemma:non-expansive}, also note that $\mathcal{P}_{\mathcal{F}}^{\mathbf{1}}(x^*)=x^*$, we have
\begin{align}
    \vert \vert x_{t+1} - x^* \vert \vert_{H_t^{-1}} &\leq \vert \vert x_{t} - x^* - \alpha_t H_t g_t \vert \vert_{H_t^{-1}} \\
    &= \Big \langle x_t - x^*, H_t^{-1} (x_t-x^*) \Big \rangle - 2 \alpha_t \Big \langle x_t - x^*, g_t \Big \rangle + \alpha_t^2 \Big \langle g_t, H_t g_t \Big \rangle
\end{align}
Hence
\begin{align}
    2 \Big \langle x_t - x^*, g_t \Big \rangle &\leq \Big \langle x_t - x^*, \frac{1}{\alpha_t} H_t^{-1} (x_t - x^*) \Big \rangle - \Big \langle x_{t+1} - x^*, \frac{1}{\alpha_t} H_t^{-1} (x_{t+1} - x^*) \Big \rangle \nonumber \\
    &+ \alpha_t \Big \langle g_t, H_t g_t \Big \rangle 
\end{align}
Perform telescope sum, we have
\begin{align}
    2 \sum_{t=1}^T \Big \langle x_t - x^* , g_t\Big \rangle & \leq \Big \langle x_1 - x^*, \frac{1}{\alpha_1} H_1^{-1} (x_1 - x^*) \Big \rangle - \Big \langle x_{T+1} - x^*, \frac{1}{\alpha_T} H_T (x_{T+1} - x^*) \Big \rangle \nonumber \\
    &+ \sum_{t=2}^T \Big \langle x_t-x^*, \Big( \frac{1}{\alpha_t} H_t^{-1} - \frac{1}{\alpha_{t-1}} H_{t-1}^{-1} \Big) \Big( x_t - x^* \Big) \Big \rangle + \sum_{t=1}^T \alpha_t \Big \langle g_t, H_t g_t \Big \rangle \\
    &\leq \Big \langle x_1 - x^*, \frac{1}{\alpha_1} H_1^{-1} (x_1 - x^*) \Big \rangle \nonumber \\
    &+ \sum_{t=2}^T \Big \langle x_t-x^*, \Big( \frac{1}{\alpha_t} H_t^{-1} - \frac{1}{\alpha_{t-1}} H_{t-1}^{-1} \Big) \Big( x_t - x^* \Big) \Big \rangle + \sum_{t=1}^T \alpha_t \Big \langle g_t, H_t g_t \Big \rangle \\
    &\leq \Big \langle x_1 - x^*, \frac{1}{\alpha_1} H_1^{-1} (x_1 - x^*) + \sum_{t=2}^T \Big \vert \Big \vert \frac{1}{\alpha_t} H_t^{-1} - \frac{1}{\alpha_{t-1}} H_{t-1}^{-1} \Big \vert \Big \vert_1 D^2 + \sum_{t=1}^T \alpha_t \Big \langle g_t, H_t, g_t\Big \rangle \\
    &\Big( \textit{Since we assume } \alpha_t \leq \alpha_{t-1}, H_t \leq H_{t-1} \textit{ element-wise. } \mathcal{F} \textit{ has bounded diameter} D.  \Big) \nonumber \\
    &\leq \langle x_1 - x^*, \frac{1}{\alpha_1} H_1^{-1} (x_1 - x^*) + D^2 \Big( \Big \vert \Big \vert \frac{1}{\alpha_T} H_{T,i}^{-1} \Big \vert \Big \vert _1 - \Big \vert \Big \vert  \frac{1}{\alpha_1} H_{1,i}^{-1} \Big \vert \Big \vert_1 \Big) + \sum_{t=1}^T \alpha_t C_u M_g^2 \\
    &\Big( \textit{By telescope sum. By assumption, $H_t$ is upper bounded }, \vert \vert g_t \vert \vert_\infty \leq M_g   \Big) \\
    &\leq \frac{1}{C_l} \Big[ \frac{1}{\alpha_1} \Big \vert \Big \vert x_1 - x^* \Big \vert \Big \vert^2 +\frac{1}{\alpha_0} D^2  T^{\eta} \Big] + C_u M_g^2 \alpha_0 \Big( \zeta(\eta)+\frac{1}{1-\eta}T^{1-\eta} + \frac{1}{2}T^{-\eta} \Big) \\
    &\Big( \textit{By sum of generalized harmonic series \cite{kronenburg2011some}}, \nonumber \\
    &\sum_{k=1}^n \frac{1}{k^s} \sim \zeta(s) + \frac{n^{1-s}}{1-s}+\frac{1}{2 n^s}  +O(n^{-s-1}), s \in (0,1), \zeta(s) \textit{ is Riemann zeta function}. \Big) \nonumber 
\end{align}
By convexity of $f_t$, we have
\begin{align}
    \mathcal{R}(T) = \sum_{t=1}^T \Big( f_t(x_t) - f_t(x^*) \Big) \leq \frac{1}{2 C_l} \Big[ \frac{1}{\alpha_1} \Big \vert \Big \vert x_1 - x^* \Big \vert \Big \vert^2 + \frac{D^2}{ \alpha_0} T^{\eta} \Big] + \frac{C_u M_g^2 \alpha_0}{2} \Big( \zeta(\eta)+\frac{1}{1-\eta}T^{1-\eta} + \frac{1}{2}T^{-\eta} \Big)
\end{align}
Equivalently,

\begin{align}
    \frac{1}{T} \sum_{t=1}^T \Big( f_t(x_t) - f_t(x^*) \Big) \leq \frac{1}{C_l} \frac{D^2}{2 \alpha_0} T^{\eta-1}+C_u \frac{M_g^2 \alpha_0}{2(1-\eta)}T^{-\eta} + O(T^{-1})
\end{align}
\end{proof}

\subsection{Convergence analysis of Async-moment-optimizers for online convex optimization}
\begin{theorem} [Thm. 3.5 in the main paper]
Under the same assumptions as in Thm.~\ref{thm:convex_bgrad_converge},
the sequence is generated by 
\begin{equation}
    x_{t+1} = \mathcal{P}_\mathcal{F}^{\mathbf{1}} \Big( x_t - \alpha_t H_t m_t \Big)
\end{equation}
where $\mathcal{P}_\mathcal{F}$ represents the projection onto convex set $\mathcal{F}$.
Then we have
\begin{align}
    \frac{1}{T}\sum_{t=1}^T (f_t(x_t)-f_t(x^*)) &\leq \frac{1}{C_l} \frac{D^2}{2\alpha_0}T^{\eta-1}+\Big[ \frac{C_u }{2} +\frac{C_u^2 \beta_1  }{1-\beta_1} \Big]\alpha_0 \frac{M_g^2}{1-\eta} T^{-\eta} + O(T^{-1})
\end{align}
\end{theorem}
\begin{proof}
Note that by definition of $m_t$, we have
\begin{align}
    g_t &= \frac{1}{1-\beta_1}m_t - \frac{\beta_1}{1-\beta_1}m_{t-1} \\
    \langle g_t, x_t - x^* \rangle &= \frac{1}{1-\beta_1} \Big( \langle m_t, x_t - x^*\rangle - \langle m_{t-1}, x_{t-1}-x^* \rangle \Big) + \langle m_{t-1}, x_{t-1}-x^* \rangle \nonumber \\
    &- \frac{\beta_1}{1-\beta_1} \langle m_{t-1}, x_t - x_{t-1} \rangle
\end{align}
By convexity of $f_t$, we have
\begin{align}
   \sum_{t=0}^T \Big( f_t(x_t) - f_t(x^*) \Big) &\leq \sum_{t=1}^T \Big \langle g_t, x_t - x^* \Big \rangle \\
    &= \frac{1}{1-\beta_1}\Big( \langle m_T, x_T-x^* \rangle - \langle m_0, x_0 -x^* \rangle \Big)+\langle m_0, x_0 - x^* \rangle \nonumber \\
    &+ \sum_{t=1}^{T-1} \langle m_t, x_t - x^* \rangle + \frac{\beta_1}{1-\beta_1} \sum_{t=1}^T \langle m_{t-1}, x_{t-1} - x_t\rangle \\
    &= \frac{\beta_1}{1-\beta_1} \langle m_T, x_T - x^* \rangle + \sum_{t=1}^T \langle m_t, x_t - x^* \rangle + \frac{\beta_1}{1-\beta_1} \sum_{t=1}^T \langle m_{t-1}, x_{t-1} -x_t \rangle
    \label{eq:rt_momen_convex}
\end{align}
where the last equality use that $m_0$ is initialized as $\vec{0}$. 
Next, we bound each term on the right hand side of Eq.~\eqref{eq:rt_momen_convex}.
First, note that by Lemma.~\ref{lemma:non-expansive},
\begin{align}
    \Big \langle x_{t+1}-x^*, H_t^{-1}(x_{t+1}-x) \Big \rangle &\leq \Big \langle x_t-x^*-\alpha_t H_t m_t, H_t^{-1} \big( x_t - x^* - \alpha_t H_t m_t \big) \Big \rangle \\
    &= \Big \langle x_t - x^*, H_t^{-1} (x_t - x^*) \Big \rangle + \alpha_t^2 \Big \langle m_t, H_t m_t \Big \rangle - 2 \alpha_t \Big \langle m_t, x_t - x^* \Big \rangle
\end{align}
Hence, we have
\begin{align}
    2 \Big \langle m_t, x_t - x^* \Big \rangle &\leq \Big \langle x_t - x^*, \frac{1}{\alpha_t} H_t^{-1} (x_t-x^*) \Big \rangle - \Big \langle x_{t+1} - x^*, \frac{1}{\alpha_t} H_t^{-1} (x_{t+1}-x^*) \Big \rangle + \alpha_t \Big \langle m_t, H_tm_t \Big \rangle
\end{align}
Perform telescope sum, we have
\begin{align}
    2 \sum_{t=1}^T \Big \langle m_t, x_t - x^* \Big \rangle &\leq \sum_{t=1}^{T}\Big( \Big \langle x_t - x^*, \frac{1}{\alpha_t} H_t^{-1} (x_t-x^*) \Big \rangle - \Big \langle x_{t+1} - x^*, \frac{1}{\alpha_t} H_t^{-1} (x_{t+1}-x^*) \Big \rangle \Big) \nonumber \\
    &+\sum_{t=1}^T \alpha_t \Big \langle m_t, H_t m_t\Big \rangle \\
    &= \Big \langle x_1 - x^*, \frac{1}{\alpha_1} H_1^{-1} (x_1 - x^*) \Big \rangle + \sum_{t=2}^T \Big \langle x_t - x^*, \big( \frac{1}{\alpha_t} H_t^{-1} - \frac{1}{\alpha_{t-1}}H_{t-1}^{-1} \big)x_t - x^*  \Big \rangle \nonumber \\
    & - \Big \langle {x_{T+1}-x^*, \frac{1}{\alpha_T}H_T^{-1}(x_{T+1}-x^*)} \Big \rangle + \sum_{t=1}^T \alpha_t \Big \langle m_t, H_t m_t \Big \rangle \\
    &\leq \Big \langle x_1 - x^*, \frac{1}{\alpha_1} H_1^{-1} (x_1 - x^*) \Big \rangle + \sum_{t=2}^T \Big \langle x_t - x^*, \Big( \Big \vert \Big \vert \frac{1}{\alpha_t} H_t^{-1} \Big \vert \Big \vert_1 - \Big \vert \Big \vert \frac{1}{\alpha_{t-1}} H_{t-1}^{-1} \Big \vert \Big \vert_1 \Big ) x_t - x^* \Big \rangle \nonumber \\
    &+ \sum_{t=1}^T \alpha_t \Big \langle m_t, H_t m_t \Big \rangle \\
    &\Big(\textit{Since } \alpha_t \leq \alpha_{t-1}, H_t \leq H_{t-1} \textit{ element-wise} \Big) \nonumber \\
    &\leq \Big \langle x_1 - x^*, \frac{1}{\alpha_1} H_1^{-1} (x_1 - x^*) \Big \rangle + D^2 \sum_{t=2}^T \Big( \Big \vert \Big \vert \frac{1}{\alpha_t} H_t^{-1} \Big \vert \Big \vert_1 - \Big \vert \Big \vert \frac{1}{\alpha_{t-1}} H_{t-1}^{-1} \Big \vert \Big \vert_1 \Big ) \nonumber \\
    &+ \sum_{t=1}^T \alpha_t \Big \langle m_t, H_t m_t \Big \rangle \\
    &\Big( \textit{Since we assume } \mathcal{F} \textit{ has bounded diameter.} \Big) \nonumber \\
    &= \Big \langle x_1 - x^*, \frac{1}{\alpha_1} H_1^{-1} (x_1 - x^*) \Big \rangle + D^2 \Big( \Big \vert \Big \vert \frac{1}{\alpha_T} H_T^{-1} \Big \vert \Big \vert_1 - \Big \vert \Big \vert \frac{1}{\alpha_1} H_1^{-1} \Big \vert \Big \vert_1 \Big) \nonumber \\
    &+ \sum_{t=1}^T \alpha_t C_u M_g^2 \\
    &\Big( \textit{ $H_t$ and $g_t$ are upper bounded by assumption.} \Big) \nonumber \\
    &\leq \frac{1}{C_l} \Big[ \frac{1}{\alpha_1}D^2 + D^2 T^{\eta} \frac{1}{\alpha_0} \Big] + C_u M_g^2 \alpha_0 \Big( \zeta(\eta)+\frac{1}{1-\eta}T^{1-\eta} + \frac{1}{2}T^{-\eta} \Big) \label{eq:rt_convex_bd1} \\
    &\Big( \textit{By sum of harmonic series} \Big) \nonumber 
\end{align}
Next, we bound $\sum_{t=1}^T \Big \langle m_{t-1}, x_{t-1}-x_t \Big \rangle$.
\begin{align}
    \sum_{t=1}^T \Big \langle m_{t-1}, x_{t-1}-x_t \Big \rangle &= \sum_{t=0}^{T-1} \Big \langle m_t, x_t - x_{t+1} \Big \rangle \\
    &\leq \sum_{t=0}^{T-1} \Big \vert \Big \vert m_t \Big \vert \Big \vert_{H_t^{1/2}} \Big \vert \Big \vert x_{t+1} - x_t \Big \vert \Big \vert_{H_t^{-1/2}} \\
    &\Big( \textit{By H\"older inequality} \Big) \nonumber \\
    &\leq \sum_{t=0}^T \Big \vert \Big \vert m_t \Big \vert \Big \vert_{H_t^{1/2}} \Big \vert \Big \vert \alpha_t H_t m_t \Big \vert \Big \vert_{H_t^{-1/2}} \\
    &\Big( x_{t+1} \textit{ is the projection of updated value onto } \mathcal{F}. \textit{ By Lemma.~\ref{lemma:non-expansive}} \Big) \nonumber \\
    &= \sum_{t=0}^T \sqrt{ \Big \langle m_t, H_t^{1/2}m_t \Big \rangle} \sqrt{ \Big \langle \alpha_t H_t m_t, \alpha_t H_t^{1/2} m_t \Big \rangle} \\
    &= \sum_{t=0}^T \alpha_t \Big \langle H_t m_t, H_t m_t \Big \rangle \\
    &\leq \alpha_0 C_u^2 M_g^2 \Big( \zeta(\eta)+\frac{1}{1-\eta}T^{1-\eta} + \frac{1}{2}T^{-\eta} \Big) \label{eq:rt_convex_bd2}
\end{align}
Finally, we have
\begin{align}
    \Big \langle m_T, x_T - x^* \Big \rangle &\leq D M_g \label{eq:rt_convex_bd3}
\end{align}
Combine Eq.~\eqref{eq:rt_momen_convex}, Eq.~\eqref{eq:rt_convex_bd1}, Eq.~\eqref{eq:rt_convex_bd2} and Eq.~\eqref{eq:rt_convex_bd3}, we have:
\begin{align}
    \sum_{t=1}^T (f_t(x_t)-f_t(x^*)) &\leq \frac{1}{2C_l} \Big[ \frac{1}{\alpha_1}D^2 + D^2 T^{\eta} \frac{1}{\alpha_0} \Big] + \frac{ C_u M_g^2 \alpha_0}{2} \Big( \zeta(\eta)+\frac{1}{1-\eta}T^{1-\eta} + \frac{1}{2}T^{-\eta} \Big) \nonumber \\
    &+ \frac{\beta_1}{1-\beta_1} \alpha_0 C_u^2 M_g^2 \Big( \zeta(\eta)+\frac{1}{1-\eta}T^{1-\eta} + \frac{1}{2}T^{-\eta} \Big) + \frac{\beta_1}{1-\beta_1} DM_g
\end{align}
Equivalently,
\begin{align}
    \frac{1}{T}\sum_{t=1}^T (f_t(x_t)-f_t(x^*)) &\leq \frac{1}{C_l} \frac{D^2}{2\alpha_0}T^{\eta-1}+\Big[ \frac{C_u }{2} +\frac{C_u^2 \beta_1  }{1-\beta_1} \Big] \alpha_0 \frac{M_g^2}{1-\eta} T^{-\eta} + O(T^{-1})
\end{align}
\end{proof}

% \paragraph{Notes} 
% \begin{enumerate}
% \item In Algo.~\eqref{algo:adam} and Algo.~\ref{algo:bgrad}, all operations between vectors are element-wise to match code. For analysis, such as Eq.~\eqref{eq:general_update} to Eq.~\eqref{eq:H_bgrad}, the formula are written in matrix-vector product (e.g. $H_t g_t$) and vector-vecctor product (e.g. $\langle g_t,g_t \rangle = g_t^\top g_t$ ).
% \item Adam and RMSProp both use $v_t$ in the denominator, with the difference that RMSProp uses $g_t$ in numerator, while Adam uses $m_t$ (the EMA of $g_t$) in numerator.
% \item The difference between RMSProp and BGrad is in the denominator, RMSProp (and Adam) uses EMA of $(g_t)^2$, while BGrad uses EMA of $(\Delta g_t)^2$. 
% \item In AsyncBelief, for the ease of analysis, $H_t^{bgrad}$ is a function of $s_{t-1}$, which is a function of $\{g_1, ... g_{t-1}\}$ but independent of $g_t$, hence
% \begin{equation}
%     \mathbb{E} (H_t^{bgrad} g_t \vert x_1, ... x_{t-1}) = H_t^{bgrad} \mathbb{E}(g_t \vert x_1, ... x_{t-1})
% \end{equation}
% For Adam and RMSProp, $H_t^{rmsprop}$ and $g_t$ are correlated, which makes it harder for analysis, but we can modify Algo.~\eqref{algo:adam} accordingly to make $H_t \perp g_t \vert x_1, ... x_{t-1}$.
% \end{enumerate}
